# Supplementary material for: Surrogate modeling for probability distribution estimation:uniform or adaptive design?
Source: arXiv:2404.07323 source file (2024-04-10)
Supplement: Supplementary file 2 [file supplementary_materials.pdf]

# Supplementary materials of “Active learning based surrogate-aided methods for full probability distribution estimation: uniform or adaptive design?”

Maijia Su<sup>a</sup>, Ziqi Wang<sup>b</sup>, Oreste Salvatore Bursi<sup>a</sup>, Marco Broccardo<sup>a</sup>

<sup>a</sup>Department of Civil, environmental and mechanical engineering, University of Trento, Trento, Italy

<sup>b</sup>Department of Civil and Environmental Engineering, University of California, Berkeley, United States

---

## 1. Benchmark Problems

This section introduces 16 benchmark examples, including 13 analytical examples (#1 ~ #13) and 3 structural examples based on FEMs (#14 ~ #16). The performance functions are provided in Table 1, and the probabilistic models together with the ranges of quantities of interest (QoI), i.e.,  $[y_{\min}, y_{\max}] = [F_Y^{-1}(10^{-3}), F_Y^{-1}(1 - 10^{-3})]$ , are presented in Table 2. The bounds  $y_{\min}$  and  $y_{\max}$  are estimated by crude MCS with  $10^6$  samples. Benchmarks #14 and #16 are two widely studied examples in the context of structural reliability. As for these two examples, this study adopts the same structural simulators and uncertainty models as the original problems, but we focus on computing the full probability distributions of the structural responses of interest rather than the failure probabilities.

Benchmark#15 studies a 10-story steel structure developed in [1] for vibration control problems. We adopt the simplified story-shear model of this structure. The model is assumed to be linearly elastic and has 5% Rayleigh damping for the first and second modes. In addition, the structure is subjected to a real ground motion, i.e., the N-S component of the 1940 El-Centro earthquake. The story parameters of this story-shear model are presented in Table 3. The probabilistic model supposes that the story masses and story stiffness follow the independent logarithmic normal distributions. The mean values of the random variables are taken as the corresponding real parameters as shown in Table 3, and the coefficients of variation are set as 0.02 for each story mass and 0.05 for each story stiffness. The total number of random variables of this benchmark is 20. We perform the analysis in MATLAB and specify the maximum story drift as the response of interest.

Table 1: Performance functions of the 16 Benchmarks

| No. | Function descriptions                                                                             | Dim. | Reference |
|-----|---------------------------------------------------------------------------------------------------|------|-----------|
| 1   | $\mathcal{M}(\mathbf{X}) = 2.5 - 0.2357(X_1 - X_2) + 0.00463(X_1 + X_2 - 20)^4$                   | 2    | [2]       |
| 2   | $\mathcal{M}(\mathbf{X}) = \sin\left(\frac{5X_1}{2}\right) + 2 - \frac{(X_1^2 + 4)(X_2 - 1)}{20}$ | 2    | [3]       |

Continued on next page

Table 1: Performance functions of the 16 Benchmarks (Continued)

| No. | Function descriptions                                                                                                                                                                                                                                         | Dim. | Reference |
|-----|---------------------------------------------------------------------------------------------------------------------------------------------------------------------------------------------------------------------------------------------------------------|------|-----------|
| 3   | $\mathcal{M}(\mathbf{X}) = \min \left\{ \begin{array}{l} 3 + 0.1(X_1 - X_2)^2 - \frac{(X_1+X_2)}{\sqrt{2}}; \\ 3 + 0.1(X_1 - X_2)^2 + \frac{(X_1+X_2)}{\sqrt{2}}; \\ (X_1 - X_2) + \frac{k}{\sqrt{2}}; (X_2 - X_1) + \frac{k}{\sqrt{2}} \end{array} \right\}$ | 2    | [4]       |
| 4   | $\mathcal{M}(\mathbf{X}) = \min\{X_1 - X_2; X_1 + X_2\}$                                                                                                                                                                                                      | 2    | [5]       |
| 5   | $\mathcal{M}(\mathbf{X}) = \min \left\{ \begin{array}{l} 2 - X_2 + \exp(-X_1^2/10) + (X_1/5)^4; \\ 3^2/2 - X_1X_2 \end{array} \right\}$                                                                                                                       | 2    | [6]       |
| 6   | $\mathcal{M}(\mathbf{X}) = 10 - \sum_{i=1}^2 (X_i^2 - 5 \cos(2\pi X_i))$                                                                                                                                                                                      | 2    | [4]       |
| 7   | $\mathcal{M}(\mathbf{X}) = \sin(X_1) + a \sin^2(X_2) + b X_3^4 \sin(X_1)$                                                                                                                                                                                     | 3    | [7]       |
| 8   | $\mathcal{M}(\mathbf{X}) = X_1 - \frac{32}{\pi X_2^3} \cdot \sqrt{\frac{X_3^2 X_4^2}{16} + X_5^2}$                                                                                                                                                            | 5    | [3]       |
| 9   | $\mathcal{M}(c_1, c_2, m, r, t_1, F_1) = 3r - \left  \frac{2F_1}{m\omega_0^2} \sin\left(\frac{\omega_0 t_1}{2}\right) \right $                                                                                                                                | 6    | [4]       |
| 10  | $\mathcal{M}(\mathbf{X}) = 1 - \frac{\sqrt{3(1-0.3^2)}}{\pi X_1 X_2^2 \cos^2 X_3} \left( \frac{X_6}{0.66} + \frac{X_5}{0.41 X_4} \right)$                                                                                                                     | 6    | [8]       |
| 11  | $\mathcal{M}(\mathbf{X}) = \left[ \frac{\frac{X_1 X_2}{\frac{X_3 (X_4 \frac{2\pi}{60})^2 (X_5^3 - X_6^3)}}{3 \times 385.82 (X_5 - X_6)}} \right]^{1/2} - 0.37473$                                                                                             | 6    | [9]       |
| 12  | $\mathcal{M}(\mathbf{X}) = 15.5910^4 - \frac{X_1 X_2^3}{2 X_2^3} \times \frac{X_4^2 - 4X_5 X_6 X_7^2 + X_4 (X_6 + 4X_5 + 2X_6 X_7)}{X_4 X_5 (X_4 + X_6 + 2X_6 X_7)}$                                                                                          | 7    | [3]       |
| 13  | $\mathcal{M}(r_w, r, T_u, H_u, T_l, H_l, L, K_w) = \frac{2\pi T_u (H_u - H_l)}{\ln(r/r_w) \left( 1 + \frac{2LT_u}{\ln(r/r_w) r_w^2 K_w} + \frac{T_u}{T_l} \right)}$                                                                                           | 8    | [10]      |
| 14  | A 2-dimensional 23 bars truss                                                                                                                                                                                                                                 | 10   | [11]      |
| 15  | A 10-floor shear structure                                                                                                                                                                                                                                    | 20   | -         |
| 16  | A 3-bays-5-floor Frame                                                                                                                                                                                                                                        | 21   | [12]      |

<sup>1</sup> Dim. refers to the dimensions of the problems

Table 2: Probabilistic models and ranges of QoI of the 16 Benchmarks

| No. | Probabilistic models                                                                    | $[y_{\min}, y_{\max}]$ |
|-----|-----------------------------------------------------------------------------------------|------------------------|
| 1   | $X_1 \sim \mathcal{N}(10, 3), X_2 \sim \mathcal{N}(10, 3), X_3 \sim \mathcal{N}(10, 3)$ | [12, 2061]             |
| 2   | $X_1 \sim \mathcal{N}(1.5, 1), X_2 \sim \mathcal{N}(1.5, 1)$                            | [-1.71, 3.41]          |
| 3   | $X_1 \sim \mathcal{N}(0, 1), X_2 \sim \mathcal{N}(0, 1)$                                | [-0.23, 3.24]          |

Continued on next page

Table 2: Probabilistic models and ranges of QoI of the 16 Benchmarks (Continued)

| No. | Probabilistic models                                                                                                                                                                                                                                                                                                                          | $[y_{\min}, y_{\max}]$ |
|-----|-----------------------------------------------------------------------------------------------------------------------------------------------------------------------------------------------------------------------------------------------------------------------------------------------------------------------------------------------|------------------------|
| 4   | $X_1 \sim \mathcal{N}(0, 1), X_2 \sim \mathcal{N}(0, 1)$                                                                                                                                                                                                                                                                                      | $[-4.67, 2.63]$        |
| 5   | $X_1 \sim \mathcal{N}(0, 1), X_2 \sim \mathcal{N}(0, 1)$                                                                                                                                                                                                                                                                                      | $[-0.70, 5.6]$         |
| 6   | $X_1 \sim \mathcal{N}(0, 1), X_2 \sim \mathcal{N}(0, 1)$                                                                                                                                                                                                                                                                                      | $[-12.6, 19.9]$        |
| 7   | $X_1 \sim \mathcal{U}(-\pi, \pi), X_2 \sim \mathcal{U}(-\pi, \pi), X_3 \sim \mathcal{U}(-\pi, \pi)$                                                                                                                                                                                                                                           | $[-9.1, 16.1]$         |
| 8   | $X_1 \sim \mathcal{U}(70, 80), X_2 \sim \mathcal{N}(39, 0.1), X_3 \sim \mathcal{G}(1342, 272.9),$<br>$X_4 \sim \mathcal{N}(400, 0.1), X_5 \sim \mathcal{N}(2.5 \times 10^5, 3.5 \times 10^4)$                                                                                                                                                 | $[0.9, 44.3]$          |
| 9   | $m \sim \mathcal{N}(1, 0.05), c_1 \sim \mathcal{N}(1, 0.1), c_2 \sim \mathcal{N}(0.1, 0.01),$<br>$r \sim \mathcal{N}(0.5, 0.05), F_1 \sim \mathcal{N}(1, 0.2), t_1 \sim \mathcal{N}(1, 0.2)$                                                                                                                                                  | $[-0.43, 1.41]$        |
| 10  | $X_1 \sim \mathcal{N}(7.0 \times 10^{10}, 3.50 \times 10^9),$<br>$X_2 \sim \mathcal{N}(2.50 \times 10^{-3}, 1.25 \times 10^{-4}),$<br>$X_3 \sim \mathcal{N}(0.524, 0.010480), X_4 \sim \mathcal{N}(0.90, 0.0225),$<br>$X_5 \sim \mathcal{N}(8.0 \times 10^4, 6.4 \times 10^3),$<br>$X_6 \sim \mathcal{N}(7.0 \times 10^4, 5.6.0 \times 10^3)$ | $[0.39, 0.725]$        |
| 11  | $X_1 \sim \mathcal{W}(0.9377, 4.59 \times 10^{-2}),$<br>$X_2 \sim \mathcal{N}(2.2 \times 10^5, 5.0 \times 10^3),$<br>$X_3 \sim \mathcal{U}(0.29, 5.8 \times 10^{-3}),$<br>$X_4 \sim \mathcal{N}(2.1 \times 10^4, 1.0 \times 10^3),$<br>$X_5 \sim \mathcal{N}(24.0, 0.5), X_6 \sim \mathcal{N}(8, 0.3)$                                        | $[-0.004, 0.170]$      |
| 12  | $X_1 \sim \mathcal{N}(350, 35), X_2 \sim \mathcal{N}(50.8, 5.08),$<br>$X_3 \sim \mathcal{N}(3.81, 0.381), X_4 \sim \mathcal{N}(173, 17.3),$<br>$X_5 \sim \mathcal{N}(9.38, 0.938), X_6 \sim \mathcal{N}(33.1, 3.31),$<br>$X_7 \sim \mathcal{N}(0.036, 0.0036)$                                                                                | $[-61008, 143310]$     |
| 13  | $r_w \sim \mathcal{U}(0.05, 0.15), r \sim \mathcal{LN}(7.71, 1.0056),$<br>$T_u \sim \mathcal{U}(63070, 115600), H_u \sim \mathcal{U}(990, 1100),$<br>$T_l \sim \mathcal{U}(63.1, 116), H_l \sim \mathcal{U}(700, 820),$<br>$L \sim \mathcal{U}(1120, 1680), K_w \sim \mathcal{U}(9855, 12045)$                                                | $[12, 230]$            |
| 14  | Refer to [11]                                                                                                                                                                                                                                                                                                                                 | $[5.2, 12.2]$          |
| 15  | Defined in this material                                                                                                                                                                                                                                                                                                                      | $[0.0121, 0.0174]$     |
| 16  | Refer to [12]                                                                                                                                                                                                                                                                                                                                 | $[0.007, 0.041]$       |

<sup>1</sup>  $\mathcal{N}$  denotes the normal distribution,  $\mathcal{LN}$  denotes the log-normal distribution,  $\mathcal{U}$  denotes the uniform distribution,  $\mathcal{G}$  denotes the Gumbel distribution and  $\mathcal{W}$  denotes the Weibull distribution.

## 2. Learning Functions

This section introduces three learning functions, serving as a supplement to Section 2.5 in the main text.

Table 3: Parameters of the 10-story steel structure in Benchmark#15

| Story | Height (m) | Story mass ( $10^5\text{kg}$ ) | Story stiffness ( $10^8\text{N/m}$ ) |
|-------|------------|--------------------------------|--------------------------------------|
| 1     | 5.49       | 2.82                           | 1.007                                |
| 2     | 3.96       | 2.76                           | 1.358                                |
| 3     | 3.96       | 2.76                           | 1.338                                |
| 4     | 3.96       | 2.76                           | 1.330                                |
| 5     | 3.96       | 2.76                           | 1.228                                |
| 6     | 3.96       | 2.76                           | 1.248                                |
| 7     | 3.96       | 2.76                           | 1.237                                |
| 8     | 3.96       | 2.76                           | 1.223                                |
| 9     | 3.96       | 2.76                           | 1.208                                |
| 10    | 3.96       | 2.76                           | 1.187                                |

### 2.1. MoV learning function

This learning function selects the points based on the maximum of variance (MoV) criteria. The MoV learning function is defined as

$$L_{\text{MoV}}(\mathbf{x}) = \sigma_{\mathcal{M}}^2(\mathbf{x}), \quad (1)$$

where  $\sigma_{\mathcal{M}}^2(\mathbf{x})$  is the prediction error/variance measured by the surrogate GP, PCE, or PCK.

### 2.2. Two-step learning function

The two-step learning function was proposed in [5]. Specifically, the first step focuses on identifying a position  $y^*$  in the range  $[y_{\min}, y_{\max}]$ . The position  $y^*$  is identified by maximizing a localized error  $W_L(y')$  centered at  $y'$ . This localized error is built by weighting the error metric in Eq.(8) in the main text (i.e., the errors formulated by the bounded surrogates  $\hat{\mathcal{M}}^k(x) = \hat{\mathcal{M}}(x) + k\sigma_{\mathcal{M}}(\mathbf{x})$ ) by a Gaussian kernel, and it reads as:

$$W_L(y') = \int_{y_{\min}}^{y_{\max}} \frac{|\hat{F}_Y^+(y) - \hat{F}_Y^-(y)|}{\min[\hat{F}_Y^0(y), 1 - \hat{F}_Y^0(y)]} e^{-\frac{(y-y')^2}{2(\sigma(y'))^2}} dy, \quad (2)$$

where the kernel parameters  $\sigma(y')$  is obtained by solving:

$$\sigma(y') = \{\sigma_{\mathcal{M}}(\mathbf{x}') \mid \mathbf{x}' = \arg \min_{\mathbf{x} \in S} |y' - \mathcal{M}(\mathbf{x})|\}. \quad (3)$$

Therefore, the threshold  $y^*$  is optimized by solving:

$$y^* = \arg \max_{y'} \frac{1}{Z(y')} W_L(y'), y' \in [y_{\min}, y_{\max}], \quad (4)$$

where the normalization coefficient  $Z(y')$  is computed by

$$Z(y') = \sqrt{2\pi}\sigma(y') \left( \Phi\left(\frac{y_{\max} - y'}{\sigma(y')}\right) - \Phi\left(\frac{y_{\min} - y'}{\sigma(y')}\right) \right), \quad (5)$$

where  $\Phi(\cdot)$  denotes the CDF of the standard Gaussian distribution. In the second step, we adopt the reliability-based learning function  $U$  proposed in [4] and it reads as:

$$L_t(\mathbf{x}) = \frac{|y^* - \hat{\mathcal{M}}(\mathbf{x})|}{\sigma_{\hat{\mathcal{M}}}(\mathbf{x})}. \quad (6)$$

### 2.3. Gradient-based learning function

The gradient-based learning function [13] is formulated by compromising global explorations and local exploitation:

$$\begin{aligned} L_g(\mathbf{x}) &= L^G(\mathbf{x}) + \omega(\mathbf{x}) \times L^L(\mathbf{x}) \\ &= \frac{D_{\min}(\mathbf{x})}{\max_{\mathbf{x} \in S} D_{\min}(\mathbf{x})} + \omega(\mathbf{x}) \times \frac{\hat{\mathcal{M}}^{nl}(\mathbf{x}|\mathcal{X}_{\min}(\mathbf{x}))}{\max_{\mathbf{x} \in S} \hat{\mathcal{M}}^{nl}(\mathbf{x}|\mathcal{X}_{\min}(\mathbf{x}))}, \end{aligned} \quad (7)$$

where  $L^G(\mathbf{x})$  and  $L^L(\mathbf{x})$  score the benefits of adding  $\mathbf{x}$  into the DoE from global and local search, respectively. Both these two scores are normalized by their corresponding highest score of the point in population  $S$ .  $\omega(\mathbf{x}) \in [0, 1]$  is a weighting function that balances the exploration and exploitation, defined as:

$$\omega(\mathbf{x}) = 1 - \frac{d(\mathbf{x}, \mathcal{X}_{\min}(\mathbf{x}))}{L_{\max}}, \quad (8)$$

where the normalized factor  $L_{\max}$  denotes the maximum Euclidean distance of points in the input DoE  $\mathcal{X}$ .  $d(\cdot, \cdot)$  is the Euclidean distance measure, and  $\mathcal{X}_{\min}(\mathbf{x}) \in \mathcal{X}$  is the point in the DoE with the minimum distance to points  $\mathbf{x} \in S$ .

The global exploration searches the sparse DoE region and favors the points with larger values of  $D_{\min}(\mathbf{x}) = d(\mathbf{x}, \mathcal{X}_{\min}(\mathbf{x}))$ , i.e., the points with maximum-minimum distances from  $\mathbf{x} \in S$  to  $\mathbf{x}' \in \mathcal{X}$ . The local exploitation targets the region with strong nonlinearity via the Taylor series expansion of the surrogate model at point  $\mathcal{X}_{\min}(\mathbf{x})$ . Specifically, the surrogate prediction is decomposed as two terms:

$$\hat{\mathcal{M}}(\mathbf{x}) = \hat{\mathcal{M}}^l(\mathbf{x}|\mathcal{X}_{\min}(\mathbf{x})) + \hat{\mathcal{M}}^{nl}(\mathbf{x}|\mathcal{X}_{\min}(\mathbf{x})), \quad (9)$$

where the first term represents the linearly first-order expansion and the second term is the non-linearly high-order residual. The second term captures the extent of nonlinear extrapolation beyond the expansion point  $\mathcal{X}_{\min}(\mathbf{x})$ . A larger contribution from this term to the total response indicates lower confidence in prediction accuracy. Therefore, the nonlinear residuals serve as an indicator used for locally refining the surrogates.

## References

- [1] Y. Ohtori, R. Christenson, B. Spencer Jr, S. Dyke, Benchmark control problems for seismically excited nonlinear buildings, *Journal of engineering mechanics* 130 (4) (2004) 366–385. [doi:10.1061/\(ASCE\)0733-9399\(2004\)130:4\(366\)](https://doi.org/10.1061/(ASCE)0733-9399(2004)130:4(366)).
- [2] F. Grooteman, An adaptive directional importance sampling method for structural reliability, *Probabilistic Engineering Mechanics* 26 (2) (2011) 134–141. [doi:10.1016/j.probengmech.2010.11.002](https://doi.org/10.1016/j.probengmech.2010.11.002).

- [3] G. I. Schueller, H. J. Pradlwarter, P.-S. Koutsourelakis, A critical appraisal of reliability estimation procedures for high dimensions, *Probabilistic engineering mechanics* 19 (4) (2004) 463–474. doi:<https://doi.org/10.1016/j.probengmech.2004.05.004>.
- [4] B. Echard, N. Gayton, M. Lemaire, AK-MCS: An active learning reliability method combining kriging and monte carlo simulation, *Structural Safety* 33 (2) (2011) 145–154. doi:[10.1016/j.strusafe.2011.01.002](https://doi.org/10.1016/j.strusafe.2011.01.002).
- [5] Z. Wang, M. Broccardo, A novel active learning-based gaussian process metamodeling strategy for estimating the full probability distribution in forward UQ analysis, *Structural Safety* 84 (2020) 101937. doi:[10.1016/j.strusafe.2020.101937](https://doi.org/10.1016/j.strusafe.2020.101937).
- [6] S.-K. Au, J. L. Beck, A new adaptive importance sampling scheme for reliability calculations, *Structural safety* 21 (2) (1999) 135–158. doi:[10.1016/S0167-4730\(99\)00014-4](https://doi.org/10.1016/S0167-4730(99)00014-4).
- [7] T. Ishigami, T. Homma, An importance quantification technique in uncertainty analysis for computer models, in: [1990] *Proceedings. First International Symposium on Uncertainty Modeling and Analysis*, IEEE, 1990, pp. 398–403. doi:[10.1109/ISUMA.1990.151285](https://doi.org/10.1109/ISUMA.1990.151285).
- [8] N. Shabakhty, N. Kazemi, M. Kia, Structural reliability assessment using improved harmony search evolutionary algorithm, in: *Proc., 2nd Iranian Conf. on Reliability Engineering*, Aerospace Research Institute Tehran, Iran, 2011, pp. 1–9.
- [9] D. Wei, S. Rahman, Structural reliability analysis by univariate decomposition and numerical integration, *Probabilistic Engineering Mechanics* 22 (1) (2007) 27–38. doi:[10.1016/j.probengmech.2006.05.004](https://doi.org/10.1016/j.probengmech.2006.05.004).
- [10] R. Schöbi, B. Sudret, S. Marelli, Rare event estimation using polynomial-chaos kriging, *ASCE-ASME Journal of Risk and Uncertainty in Engineering Systems, Part A: Civil Engineering* 3 (2) (2017) D4016002. doi:[10.1061/AJRUA6.0000870](https://doi.org/10.1061/AJRUA6.0000870).
- [11] G. Blatman, B. Sudret, Efficient computation of global sensitivity indices using sparse polynomial chaos expansions, *Reliability Engineering & System Safety* 95 (11) (2010) 1216–1229. doi:[10.1016/j.strusafe.2018.06.003](https://doi.org/10.1016/j.strusafe.2018.06.003).
- [12] P. Liu, Der kiureghian: A. optimization algorithms for structural reliability, *Structural Safety* 9 (3) (1991) 161–177. doi:[10.1016/0167-4730\(91\)90041-7](https://doi.org/10.1016/0167-4730(91)90041-7).
- [13] S. Mo, D. Lu, X. Shi, G. Zhang, M. Ye, J. Wu, J. Wu, A taylor expansion-based adaptive design strategy for global surrogate modeling with applications in groundwater modeling, *Water Resources Research* 53 (12) (2017) 10802–10823. doi:[10.1002/2017WR021622](https://doi.org/10.1002/2017WR021622).
